# Supplementary material for: Accurate Column Moist Static Energy Budget in Climate Models. Part 1: Conservation Equation Formulation, Methodology, and Primary Results Demonstrated Using GISS ModelE3
Source: arXiv:2407.13855 source file (2025-11-25)
Supplement: Supplementary file 1 [file 2024_MSE_budget_part1_SI.pdf]

# Supporting Information for “Accurate Column Moist Static Energy Budget in Climate Models. Part 1: Conservation Equation Formulation, Methodology, and Primary Results Demonstrated Using GISS ModelE3”

Kuniaki Inoue<sup>1,2</sup>, Maxwell Kelley<sup>2</sup>, Ann M. Fridlind<sup>2</sup>, Michela Biasutti<sup>3</sup>,

Gregory S. Elsaesser<sup>2,4</sup>

<sup>1</sup>Center for Climate System Research, Columbia University, New York, NY, USA

<sup>2</sup>NASA Goddard Institute for Space Studies, New York, NY, USA

<sup>3</sup>Lamont-Doherty Earth Observatory, Columbia University, Palisades, NY, USA

<sup>4</sup>Department of Applied Physics and Mathematics, Columbia University, New York, NY, USA

## Contents of this file

1. Figure S1

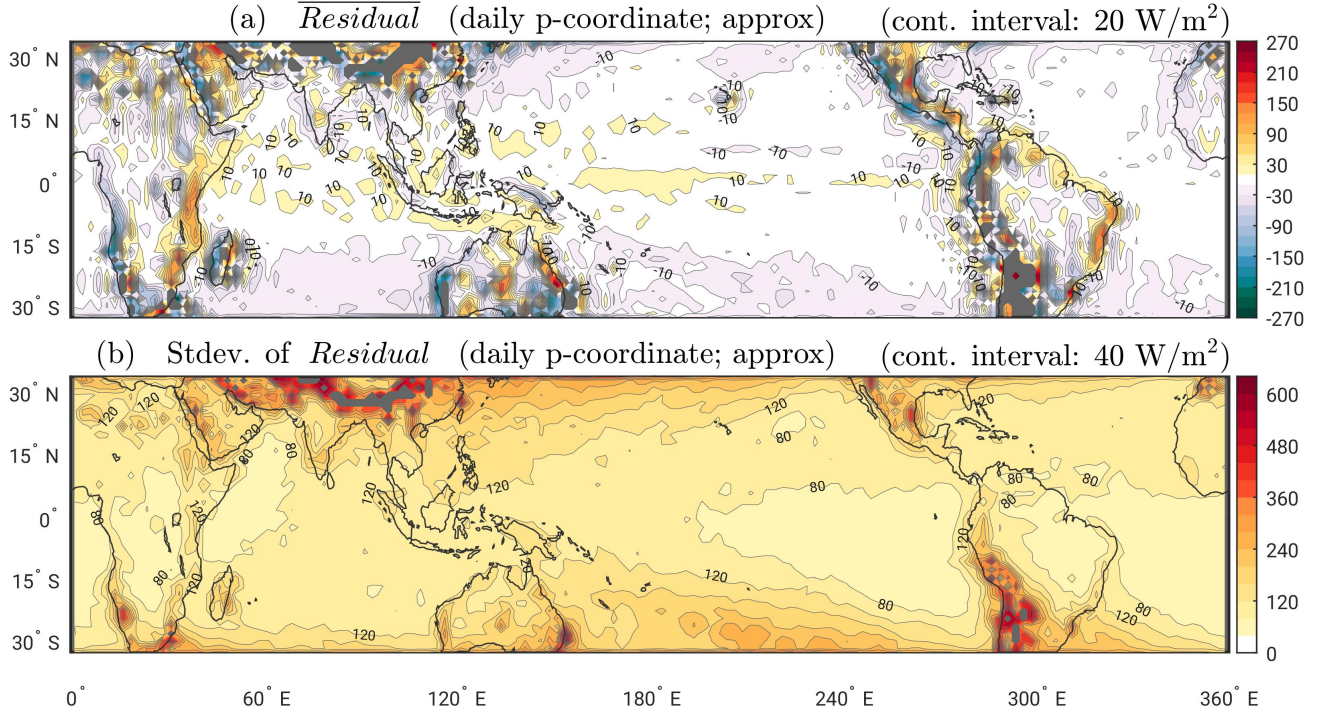

**Figure S1.** Similar to Fig. 1(a) and (c), but the residual is computed using the approximated column MSE budget equation (Eq. 16). The domain average for Panel (a) is  $-5.8322 \text{ W m}^{-2}$ , slightly lower than the  $-5.6151 \text{ W m}^{-2}$  observed in Fig. 1(a). This indicates that the approximation of the MSE budget equation slightly increases the magnitude of the residual, although the difference is negligible.
